# Supplementary material for: From the Hardness of Detecting Superpositions to Cryptography: Quantum Public Key Encryption and Commitments
Source: arXiv:2210.05978 source file (2023-04-23)
Supplement: Supplementary file 1 [file Appendix_Lattices.tex]

\subsection{Quantum-Ciphertext Public Key Encryption from Lattices}\label{sec:Lattices}
%In the previous subsections, we construct a quantum-ciphertext PKE scheme based on cryptographic group actions. 
Here, we describe two lattice-based constructions of quantum-ciphertext PKE schemes based on similar ideas to the one in \Cref{sec:QPKE_construction}. Both constructions are based on the hardness of the LWE problem.
Since it is already known how to construct classical PKE schemes based on LWE \cite{JACM:Regev09,STOC:GenPeiVai08}, this does not give a new feasibility result unlike the group action-based one. Thus, we only give sketches for them. \takashi{Do you think this is okay? We may move it to appendix.}
%generalize the construction to be based on broader class of assumptions. 

\smallskip
\noindent\textbf{First construction.}
Our first construction is based on noisy trapdoor claw-free family (NTCF) based on LWE constructed in \cite{FOCS:BCMVV18}. For ease of presentation, we assume non-noisy ideal trapdoor claw-free permutations. A similar construction works with NTCFs by similar techniques as in  \cite{FOCS:BCMVV18}. %We will directly describe a quantum PKW scheme without going through equivocal commitments though the idea is similar.

A trapdoor claw-free permutation consists of two permutations $f_0$ and $f_1$ over a set $X$. As claw-freeness we require that it is hard to find $x_0$ and $x_1$ such that $f_0(x_0)=f_1(x_1)$. On the other hand, if one is given a trapdoor, one can find $x_0$ and $x_1$ such that $f(x_0)=f(x_1)=y$ for any given $y$.

Using it, we construct computationally binding and equivocal canonical quantum bit commitments as follows. 
\begin{itemize}
\item $\setup(1^\secp)$ generates a trapdoor claw-free permutation
$(f_0,f_1)$ along with the corresponding trapdoor $\td$ and outputs $\pp\seteq (f_0,f_1)$ and $\td$. 
\item For $\pp=(f_0,f_1)$ and $\td$, $Q_{\pp,b}$ is defined so that we have 
\begin{align*}
    Q_{\pp,b}\ket{0}_{\regC,\regR}=\frac{1}{|X|^{1/2}}\sum_{x\in X}\ket{f_b(x)}_{\regC}\ket{x}_{\regR}.
\end{align*}
\end{itemize}

For $\td$, we define $U_{\td,\regR}$ by
\begin{align*}
U_{\td,\regR}\ket{x}_{\regR}\seteq \ket{f_1^{-1}(f_0(x))}_\regR.   
\end{align*}  
\mor{ancilla is not necessary, like $U_{\td,\regR}|x\rangle|0\rangle|0\rangle=|x\rangle|f^{-1}_1(f_0(x))\rangle|junk\rangle$?}
Then, it is easy to see that it meets the definition of equivocality.  
%Indeed, we have 
%\begin{align*}
%&\left|\bra{0}_{\regC,\regR}Q_{\pp,1}^\dagger(I_{\regC}\otimes U_{\td,\regR}) Q_{\pp,0}\ket{0}_{\regC,\regR}\right|
%\end{align*}

For proving the computational binding property, suppose that it is not computationally binding. Then, there is a \mor{polynomial-time computable?} unitary $U_\pp$ over $(\regR,\regZ)$ and an auxiliary state $\ket{\tau}_{\regZ}$ such that 
\begin{align*}
    \mathbb{E}\left[\left\|(Q_{\pp,1}\ket{0}\bra{0}Q_{\pp,1}^\dagger)_{\regC,\regR}(I_{\regC}\otimes U_{\pp,\regR,\regZ})((Q_{\pp,0}\ket{0})_{\regC,\regR}\ket{\tau}_{\regZ})\right\|\right]
\end{align*}
is non-negligible 
where $\pp=(f_0,f_1)$ for a randomly generated $(f_0,f_1)$. 
Then, we construct a non-uniform QPT algorithnm $\A$ with advice $\ket{\tau}$ that breaks the claw-freeness of $(f_0,f_1)$ as follows:

\begin{description}
\item[$\A((f_0,f_1);\ket{\tau})$:] Given the problem instance $(f_0,f_1)$ and advice $\ket{\tau}_{\regZ}$, uniformly pick $x_0\in X$, apply $U_{\pp}$ to $\ket{x_0}_{\regR}\ket{\tau}_{\regZ}$, measure $\regR$ to get $x'_1$, and output $(x_0,x'_1)$.  
\end{description}

Let $x_1\seteq f^{-1}_1(f_0(x_0))$. Our goal is to prove that $x'_1 = x_1$ with a non-negligible probability. This can be proven as follows.
\begin{align*}
    &\Pr[x'_1=x_1:x'_1 \gets \A(f_0,f_1;\ket{\tau})]\\
    &=\mathbb{E}\left[\frac{1}{|X|}\sum_{x_0\in X}\left\|\bra{x_1}_{\regR}U_{\pp,\regR,\regZ}\ket{x_0}_{\regR}\ket{\tau}_{\regZ}\right\|^2\right]\\
    &\geq 
    \mathbb{E}\left[\frac{1}{|X|^2}\left(\sum_{x_0\in X}\left\|\bra{x_1}_{\regR}U_{\pp,\regR,\regZ}\ket{x_0}_{\regR}\ket{\tau}_{\regZ}\right\|\right)^2\right]\\
    &\geq \mathbb{E}\left[\frac{1}{|X|^2}\left\|\sum_{x_0\in X}\bra{x_1}_{\regR}U_{\pp,\regR,\regZ}\ket{x_0}_{\regR}\ket{\tau}_{\regZ}\right\|^2\right]\\
    &\geq \mathbb{E}\left[\frac{1}{|X|}\left\|\sum_{x_0\in X}\bra{x_1}_{\regR}U_{\pp,\regR,\regZ}\ket{x_0}_{\regR}\ket{\tau}_{\regZ}\right\|\right]^2\\
    &=\mathbb{E}\left[
    \frac{1}{|X|}
    \left\|\left(\sum_{x_1\in X}\bra{f_1(x_1)}_{\regC}\bra{x_1}_{\regR}\right)
    \left(I_\regC\otimes U_{\pp,\regR,\regZ}\right)
     \left(\sum_{x_0\in X}\ket{f_0(x_0)}_{\regC}\ket{x_0}_{\regR}\right)\right\|
    \right]^2\\
    &= \mathbb{E}\left[\left\|(Q_{\pp,1}\ket{0}\bra{0}Q_{\pp,1}^\dagger)_{\regC,\regR}(I_{\regC}\otimes U_{\pp,\regR,\regZ})((Q_{\pp,0}\ket{0})_{\regC,\regR}\ket{\tau}_{\regZ})\right\|\right]^2.
\end{align*}
%where the first inequality follows from Cauchy–Schwarz inequality  and the second inequality follows from the triangle inequality.
By the assumption, this is non-negligible. Thus, $\A$ finds a claw with a non-negligible probability, which contradicts the claw-freeness. Therefore, the above commitment scheme is computationally binding.

Now, we obtain an equivocal and computationally binding canonical bit quantum commitments with setup.
By \Cref{cor:QPKE_and_equ}, this immediately leads to IND-CPA secure quantum PKE. Concretely, the scheme is as follows. 
The public key is $\pk=(f_0,f_1)$, the secret key is its trapdoor $\sk=\td$, and the ciphertext for a bit $b\in \bit$ is 
\begin{align*}
    \qct_b=\frac{1}{\sqrt{2}}\left(\ket{0}\ket{x_0}+(-1)^b\ket{1}\ket{x_1}\right)
\end{align*}
where $f_0(x_0)=f_1(x_1)=y$ for a uniformly random $y\in X$. 
\mor{$y$ is also contained in the ciphertext?}
\mor{I do not understand why this $\qct_b$ is equal to $\Tr_\regR(Q_{pp,b}|0\rangle_{\regC,\regR})$.}
\minki{I think a more detail would be helpful; the overall ciphertext-randomness (for construct ciphertext) pairs is of the form $\sum_{x\in X}\ket{f_0(x)}\ket{0,x} \pm \ket{f_1}\ket{1,x}= \sum_{y \in Y} \ket{y} \left(\ket {0,x_0} \pm \ket{1,x_1}\right)$ where $f_0(x_0)=f_1(x_1)=y.$ Here the first register (=$\regC$) is a sort of randomness for constructing the ciphertext; one who did encrypt holds this register, and do not need to publish this register at all, thus we can trace out $\regC.$}

\begin{remark}[On the trapdoor.]
It is worth mentioning that we actually do not need the full power of $\td$. For the decryption,  we do not need to recover $(x_0,x_1)$ from $y$. We only need a trapdoor that enables us to compute $x_0$ from $x_1$ and $x_1$ from $x_0$. In the LWE-based construction (with noises)~\cite{FOCS:BCMVV18}, this is very easy because we always have $x_1 = x_0 -s \mod q$ for some secret vector $s$ which corresponds to the LWE secret. Thus, the secret key of the above quantum-ciphertext PKE scheme can be set to be the LWE secret rather than so called ``lattice trapdoors''~\cite{STOC:GenPeiVai08,C:MicPei13}.  
\end{remark}
\begin{remark}[On Ring-LWE]
We do not use the ``adaptive hardcore'' property, which \cite{FOCS:BCMVV18} introduced and showed that the LWE-based construction satisfies. Thus, we can also use the Ring-LWE based construction of NTCFs given in \cite{BKVV20}, which gives more efficient construction than the LWE-based one (though our focus in this paper is not on the actual efficiency).
\end{remark}

\if0
Using it, we construct quantum PKE scheme as follows.

\begin{description}
\item[$\keygen(1^\secp)$:] 
Sample $(f_0,f_1)$ along with trapdoor $\td$. 
Output $\pk\seteq (f_0,f_1)$ and $\sk \seteq \td$. 
\item[$\enc(\pk,b\in \bit)$:] 
Output a ciphertext 
\begin{align*}
    \ct\seteq  \frac{1}{\sqrt{2}}(\ket{0}\ket{x_0}+(-1)^b\ket{1}\ket{x_1})
\end{align*}
where $f(x_0)=f(x_1)=y$ for uniformly random $y$. 

We note that such a state can be generated as follows using the technique of \cite{FOCS:BCKMM18}.
Generate a state  
\begin{align*}
    \frac{1}{\sqrt{2}}(\ket{0}+(-1)^b\ket{1})\frac{1}{|X|^{1/2}}\sum_{x\in X}\ket{x}
\end{align*}
coherently compute $f_0$ or $f_1$ controlled by the first qubit in an additional register to get 
\begin{align*}
    \sum_{x\in X}\frac{1}{(2|X|)^{1/2}}\ket{0}\ket{x}\ket{f_0(x)}+(-1)^b \ket{1}\ket{x}\ket{f_1(x)}),
\end{align*}
and measure the rightmost register to get $y$. At this point, the first two registers collapse to \begin{align*}
    \frac{1}{\sqrt{2}}(\ket{0}\ket{x_0}+(-1)^b \ket{1}\ket{x_1}),
\end{align*}
where where $f(x_0)=f(x_1)=y$. 
\item[$\dec(\sk,\ct)$:] 
Let $\regD$ and $\regX$ be the first and second registers of $\ct$, respectively. 
Prepare $\ket{+}_\regB=\frac{1}{\sqrt{2}}(\ket{0}+\ket{1})_\regB$ in an additional one-qubit register $\regB$. 
Let $U_\td$ be a unitary over $\regD$ and $\regG$ such that 
\begin{align*}
    &U_\td \ket{0}_{\regD} \ket{x_0}_{\regX} = \ket{1}_{\regD}\ket{x_1}_{\regX}, \\
    &U_\td \ket{1}_{\regD}\ket{x_1}_{\regX} = \ket{0}_{\regD}\ket{x_0}_{\regX}
\end{align*}
for any $x_0,x_1$ such that $f_0(x_0)=f_1(x_1)$. 
Apply the controlled-$U_\td$ controlled by $\regB$.
Finally, measure $\regB$ in the Hadamard basis and output the measurement outcome $b'$. (See Figure ?? \takashi{to be written.})
\end{description}

Correctness can be seen by an easy calculation.
Security is proven as follows. Suppose that the above scheme is not IND-CPA secure. Then, by \Cref{item:binding_to_hiding_setup} of \Cref{thm:conversion_setup} 
where we think of quantum PKE as computationally hiding commitments as in \Cref{sec:equivalence_ext_and_QPKE}, there is a unitary $U_{f_0,f_1}$ that depends on the descriptions of $(f_0,f_1)$ (but not on $\td$) such that 
\begin{align*}
    \mathbb{E}\left[\left|\frac{1}{|X|}\sum_{y\in X}\bra{x_1}U_{f_0,f_1}\ket{x_0}\right|\right]
\end{align*}
is non-negligible 
where the expectation is over the choice of $((f_0,f_1),\td)$ and $x_b\defeq f^{-1}_b(y)$ for $b\in \bit$. 
By using such $U_{f_0,f_1}$, we can find a claw as follows. Given $(f_0,f_1)$, we randomly pick $x_0\in X$, generate $U_{f_0,f_1}\ket{x_0}$ and measure to get $x'_1$. Then the probability that we have $x'_1=x_1$ (where $x_1\seteq f^{-1}_1(f_0(x_0))$) is
\begin{align*}
    &\mathbb{E}\left[\frac{1}{|X|}\sum_{y\in X}\left|\bra{x_1}U_{f_0,f_1}\ket{x_0}\right|^2\right]\\
    &\geq \mathbb{E}\left[\frac{1}{|X|^2}\left|\sum_{y\in X}\bra{x_1}U_{f_0,f_1}\ket{x_0}\right|^2\right]\\
    &\geq \mathbb{E}\left[\left|\frac{1}{|X|}\sum_{y\in X}\bra{x_1}U_{f_0,f_1}\ket{x_0}\right|\right]^2.
\end{align*}
Since this is non-negligible, we can find a claw with a non-negligible probability, which contradicts the claw-freeness. Thus, the above scheme is IND-CPA secure.
\fi

%we only have to construct computationally binding and equivocal canonical quantum commitments with setup. Thus, it is natural to start from classical constructions of equivocal commitments and then ask if they can be extended to the quantum setting. As mentioned in \Cref{sec:ext_and_equ}, this does not work in general. On the other hand, it works for some constructions. Indeed, the group action-based construction is a quantum analog of the classical equivocal commitments of \Cref{C:BraYun90}.

%Here, we focus on the classical equivocal commitments from sigma-protocols with certain properties given in ??. \takashi{need to look for the citation}Roughly, a sigma-protocol (with one-bit challenge) works as follows:

\smallskip
\noindent\textbf{Second construction.}
%The SIS problem with parameters $(n,q,\beta,m)$ 
$\SIS_{n,q,\beta,m}$ is a problem to find a vector $\vz \in \ZZ_q^m\setminus \{0\}$ such that $A\vz=0$ and $\|\vz\|\leq \beta$ given $A\gets \ZZ^{n\times m}_q$. It is known that the SIS problem is at least as hard as some worst-case lattice problems~\cite{STOC:Ajtai96} under a certain parameter regime. 

Let $g_A:[-B,B]^m \rightarrow \ZZ_q^n$ be a function defined by $g_A(\vx)=A\vx$. It is easy to see that $g_A$ is collision-resistant 
if $\SIS_{n,q,\beta,m}$ is hard for $\beta\geq 2B\sqrt{m}$. Moreover, Liu and Zhandry~\cite{EC:LiuZha19} showed that $g_A$ is collapsing~(\Cref{def:collapsing}) under a certain parameter regime assuming the hardness of LWE. Recall that the collapsing property roughly means that QPT algorithms cannot distinguish if a superposition of preimages of some target value was measured or not. %(See \cite{EC:Unruh16,EC:LiuZha19} for details.)
\mor{If the definition of collapsing will be provided elsewhere in this paper, point it.}

We construct an equivocal canonical quantum bit commitments with setup based on the collapsing property of $g_A$ as follows. Let $B$ and $B'$ be positive integers such that $B>>B'$, \mor{$\gg$?}$(2B')^m >> q^n$, and $\beta>(2B+B')\sqrt{m}$.

\begin{itemize}
\item $\setup(1^\secp)$ generates 
$A\gets \ZZ_q^{n\times m}$ and 
$\vs \gets [-B',B']^m$, sets $\vt\seteq A \vs$, and outputs $\pp\seteq (A,\vt)$ and $\td\seteq \vs$. 
%e remark that $\vt$ is almost uniformly distributed over $\ZZ_q^n$ by $(2B')^m >q^n 2^\secp$ and the leftover hash lemma.
\item For $\pp=(A,\vt)$ and $\td\in \vs$\mor{$=$?}, $Q_{\pp,b}$ is defined so that we have 
\begin{align*}
    Q_{\pp,b}\ket{0}_{\regC,\regR}=\frac{1}{(2B)^{m/2}}\sum_{\vx\in [-B,B]^m}\ket{A\vx + b\vt}_{\regC}\ket{\vx}_{\regR}.
\end{align*}
\end{itemize}

For $\td=\vs$, we define $U_{\td,\regR}$ by
\begin{align*}
U_{\td,\regR}\ket{\vx}_{\regR}\seteq \ket{\vx-\vs}_{\regR}.    
\end{align*}  
Then, we can show that it meets the definition of equivocality assuming that $B/B'$ is super-polynomial.

For proving the computational binding property, suppose that it is not computationally binding. Then, there is a \mor{polynomial-time computable?} unitary $U_\pp$ over $(\regR,\regZ)$ and an auxiliary state $\ket{\tau}_{\regZ}$ such that 
\begin{align*}
    \mathbb{E}\left[\left\|(Q_{\pp,1}\ket{0}\bra{0}Q_{\pp,1}^\dagger)_{\regC,\regR}(I_{\regC}\otimes U_{\pp,\regR,\regZ})((Q_{\pp,0}\ket{0})_{\regC,\regR}\ket{\tau}_{\regZ})\right\|\right]
\end{align*}
is non-negligible 
where $A\gets \ZZ_q^{n\times m}$, $\vs\gets [-B',B']^m$, 
$\vt\seteq A\vs$, and $\pp\seteq (A,\vt)$. %Note that we used the fact that the distribution of $\vt$ is almost uniform here. 

Then, we can construct a non-uniform QPT algorithm $\A$ with advice $\ket{\tau}$ that solves $\SIS_{n,q,m,\beta}$ as follows. 
\begin{description}
\item[$\A(A;\ket{\tau})$]
Given the problem instance $A\in \ZZ_q^{n\times m}$ and advice $\ket{\tau}$, randomly pick $\vs \gets [-B',B']^m$ and $\vx\gets [-B,B]^m$, 
set $\vt\seteq A\vs$ and $\pp \seteq (A,\vt)$, 
apply $U_\pp$ on
$\ket{\vx}_{\regR}\ket{\tau}_{\regZ}$, measure $\regR$ to get $\vx'$, and output $\vx-\vx'-\vs$. 
\end{description}

First, we show that we have $A\vx'+ \vt=A\vx$ and $\vx'\in [-B,B]^m$ with non-negligible probability. This can be seen as follows. If we replace $\ket{\vx}_{\regR}\ket{\tau}_{\regZ}$ with a state $\propto \sum_{\vx''\in [-B,B]^m:A\vx''=A\vx}\ket{\vx''}_{\regR}\ket{\tau}_{\regZ}$, the above directly follows from the assumption that $U_\pp$ breaks binding by a similar calculation to that for the first construction above. Then, by the assumption that $g_A$ is collapsing, the probability that $A\vx'+ \vt=A\vx$ and $\vx'\in [-B,B]^m$ is still non-negligible even if we use $\ket{\vx}_{\regR}\ket{\tau}_{\regZ}$ instead of $\propto \sum_{\vx''\in [-B,B]^m:A\vx''=A\vx}\ket{\vx''}_{\regR}\ket{\tau}_{\regZ}$ as is done by $\A$. When this happens, we have $A(\vx-\vx'-\vs)=0$ and $\vx-\vx'-\vs\in [-2B-B',2B+B']^m$ and in particular $\left|\vx-\vx'-\vs\right|\leq  (2B+B')\sqrt{m}\leq \beta$. Therefore, this is a valid solution to $\SIS_{n,q,m,\beta}$ if $\vx-\vx'-\vs\neq 0$. We can see that the probability that  $\vx-\vx'-\vs= 0$ is negligible: Remark that the only information of $\vs$ that is used for generating $\vx'$ is $\vt=A\vs$, which significantly loses the information of $\vs$ by $(2B')^m >> q^n$. Therefore, it is information theoretically impossible for it to output $\vx'$ such that $\vx-\vx'-\vs= 0$ with a non-negligible probability. In summary, it solves $\SIS_{n,q,m,\beta}$ with a non-negligible probability, and the proof is finished.

Now, we obtain an equivocal and computationally binding canonical bit quantum commitments with setup.
By \Cref{cor:QPKE_and_equ}, this immediately leads to IND-CPA secure quantum-ciphertext PKE. Concretely, the scheme is roughly as follows. 
The public key is $\pk=(A,\vt = A\vs)$, the secret key is $\sk=\vs$, and the ciphertext for a bit $b\in \bit$ is 
\begin{align*}
    \qct_b=\frac{1}{\sqrt{2}}\left(\ket{0}\ket{\psi_{0,\vy}}+(-1)^b\ket{1}\ket{\psi_{1,\vy}}\right)
\end{align*}
where $\vy\in \ZZ_q^n$ is almost uniformly distributed over $\ZZ_q^n$, and $\ket{\psi_{b',\vy}}$ is a uniform superposition over all $\vx\in [-B',B']^m$ such that $A\vx + b' \vt = \vy$.
