# Supplementary material for: From the Hardness of Detecting Superpositions to Cryptography: Quantum Public Key Encryption and Commitments
Source: arXiv:2210.05978 source file (2023-04-23)
Supplement: Supplementary file 2 [file Appendix_QPKE.tex]

\section{Omitted Contents in \Cref{sec:conversion}}
\subsection{Definition of Canonical Quantum Bit Commitments with Setup}\label{sec:QCom_setup}
We give a formal definition of canonical quantum bit commitments with setup.

\begin{definition}[Canonical quantum bit commitments with setup]\label{def:canonical_com_setup}
A canonical quantum bit commitment with setup scheme is represented by a PPT algorithm $\setup$ 
that takes the security parameter $1^\secp$ as input and outputs a public parameter $\pp$ and trapdoor $\td$ and
an ensemble of unitary $\{Q_{\pp,0}(\secp),Q_{\pp,1}(\secp)\}_{\secp\in \mathbb{N},\pp}$ (where $\pp$ takes over all possible values generated by $\setup(1^\secp)$) over two registers $\regC$ (called the commitment register) and $\regR$ (called the reveal register) that can be uniformly generated in polynomial-time.\mor{just saying polynomial-time computable unitary?}\footnote{Precisely speaking, we mean that there is a uniform QPT machine that generates a description of $Q_{\pp,b}(\secp)$ on input $\pp$, $b$, and $1^\secp$.} 
%We require that $Q_0\ket{\phi}_{\regC,\regR}$ and $Q_1\ket{\phi}_{\regC,\regR}$ are orthogonal for all states $\ket{\phi}_{\regC,\regR}$. 
In the rest of the paper, we often omit $\secp$ and simply write $Q_{\pp,0}$ and $Q_{\pp,1}$ to mean $Q_{\pp,0}(\secp)$ and $Q_{\pp,1}(\secp)$. 
\end{definition}

%\begin{remark}[On the Orthogonality Condition]
%The original definition in  \cite{Yan20} does not require that $Q_0\ket{\phi}_{\regC,\regR}$ and $Q_1\ket{\phi}_{\regC,\regR}$ are orthogonal. However, this can be assumed without loss of generality. Indeed, if this assumption is not satisfied, we can augment $\regR$ by a single-qubit register $\regD$ and then define an alternative scheme  $\{Q'_0(\secp),Q'_1(\secp)\}_{\secp\in \mathbb{N}}$ so that 
%\begin{align}
%    Q'_b\ket{\phi}_{\regC,\regR}\ket{d}_{\regD}=(Q_b\ket{\phi}_{\regC,\regR})\ket{d\oplus b}_{\regD}.
%\end{align}
%It is also easy to see that this conversion preserves hiding and binding properties. 
%We assume the orthogonality condition for convenience in the presentation of our duality theorem.
%\end{remark}

\begin{definition}[Hiding; with setup]
We say that a canonical quantum bit commitment with setup scheme $(\setup,\{Q_{\pp,0},Q_{\pp,1}\})$ is computationally (rep. statistically) hiding if for any non-uniform QPT (resp. unbounded-time) algorithm $\A$, we have
\begin{align*}
    \left|\Pr[\A(\pp,\Tr_{\regR}(Q_{\pp,0}\ket{0}_{\regC,\regR}))=1]- \Pr[\A(\pp,\Tr_{\regR}(Q_{\pp,1}\ket{0}_{\regC,\regR}))=1]\right|=\negl(\secp),
\end{align*}
where $(\pp,\td)\gets \setup(1^\secp)$. 
We say that it is perfectly hiding if the LHS is $0$ for all unbounded-time $\A$.
\end{definition}

\begin{definition}[Binding; with setup]
We say that a canonical quantum bit commitment with setup scheme $(\setup,\{Q_{\pp,0},Q_{\pp,1}\})$ is computationally (rep. statistically) binding if for any polynomial-time  (resp. unbounded-time) unitary $U_\pp$ (that depends on $\pp$) over $\regR$ and an additional register $\regZ$ and any polynomial-size state $\ket{\tau}_{\regZ}$, 
it holds that 
\begin{align*}
    \mathbb{E}_{(\pp,\td)\gets \setup(1^\secp)}\left\|(Q_{\pp,1}\ket{0}\bra{0}Q_{\pp,1}^\dagger)_{\regC,\regR}(I_{\regC}\otimes U_{\pp,\regR,\regZ})((Q_{\pp,0}\ket{0})_{\regC,\regR}\ket{\tau}_{\regZ})\right\|=\negl(\secp).
\end{align*}
We say that it is perfectly hiding if the LHS is $0$ for all unbounded-time unitary $U_{\pp}$. 
\end{definition}

%\subsection{Proof of \Cref{lem:ext_equ_to_binding_hiding}}\label{sec:proof_ext_equ_to_binding_hiding}
%\begin{proof}[Proof of \Cref{lem:ext_equ_to_binding_hiding}]
%Obvious \takashi{to be revised}
%\end{proof}

\subsection{Equivalence between 
Extractable Commitments and
Quantum-Ciphertext Public Key Encryption}\label{sec:equivalence_ext_and_QPKE}
We prove \Cref{lem:QPKE_and_ext}, i.e., show that extractable and computationally hiding quantum bit commitments and quantum PKE are equivalent.
\takashi{This subsection might be too tautological. Should we remove it?}
\mor{For me, it is useful.}

\smallskip
\noindent\textbf{From extractable commitments to quantum-ciphertext PKE.}
Let $(\setup,\{Q_{\pp,0},Q_{\pp,1}\})$ be a computationally hiding extractable canonical quantum bit commitment with setup. Let $\extractor$ be the corresponding extractor. Then, we construct a quantum-ciphertext PKE scheme as follows.
\begin{description}
\item[$\keygen(1^\secp)$:] 
Run $(\pp,\td)\gets \setup(1^\secp)$ and output $\pk\seteq \pp$ and $\sk \seteq \td$. 
\item[$\enc(\pk,b)$:] 
Given $\pk=\pp$ and $b\in \bit$, 
output $\qct\seteq \Tr_{\regR}(Q_{\pp,b}\ket{0}_{\regC,\regR})$. 
\item[$\dec(\sk,\qct)$:]
Given $\sk=\td$ and $\qct$, 
output $b'\gets \extractor(\td,\qct)$.
\end{description}

The correctness and IND-CPA security of the above quantum-ciphertext PKE scheme immediately follows from the extractability and the computational hiding property of the commitment scheme, respectively.

\smallskip
\noindent\textbf{From quantum-ciphertext PKE to extractable commitments.}
Let $(\keygen,\enc,\dec)$ be an IND-CPA secure quantum-ciphertext PKE scheme. By deferring all internal measurements, for any public key $\pk$ and $b\in \bit$, 
we can define a unitary $U^{\mathrm{enc}}_{pk,b}$ over registers $\regCT$ (the ciphertext register) and $\regAux$ (the auxiliary register) so that $U^{\mathrm{enc}}_{pk,b}\ket{0}_{\regCT,\regAux}=\enc(\pk,b)$. 
\mor{Do you mean
$\Tr_{\regAux}(U^{\mathrm{enc}}_{pk,b}\ket{0}_{\regCT,\regAux})=\enc(\pk,b)$ 
?}
Let $\setup$ be the same as $\keygen$ except that it renames $\pk$ and $\sk$ to $\pp$ and $\td$, respectively. Let $Q_{\pp,b} \seteq ^{\mathrm{enc}}_{pk,b}$ \mor{$U$ is forgotten?} where $\pp=\pk$ under the above renaming. Then $(\setup,\{Q_{\pp,0},Q_{\pp,1}\})$ is a computationally hiding extractable commitment. Indeed, the computational hiding property and extractability immediately follows from the IND-CPA security and correctness of the quantum-ciphetext PKE scheme.

\subsection{Proof of \Cref{lem:Gap_OW_and_EOW}}\label{sec:proof_Gap_OW_and_EOW}
We give a proof of \Cref{lem:Gap_OW_and_EOW}. Before giving the proof, we clarify definitions of terms that appear in the statement of the lemma. First, we define (infinitely-often) uniform extended one-wayness for group actions.
\begin{definition}[(Infinitely-often) uniform extended one-wayness]\label{def:ex_one-way_uniform}
We say that a group action $(G,S,\star)$ with efficient algorithms is uniform extended one-way if for any uniform QPT adversary $\A$, we have 
\begin{align*}
    \Pr\left[
    h'\star t = h\star s
    :
    \begin{array}{l}
     s\gets S,
    g,h\gets G,
    t  := g \star s,
    h' \leftarrow \A(s,t,\ket{hG_s})
    \end{array}
    \right]=\negl(\secp).
\end{align*}
We say that it is infinitely-often uniform extended one-way if the above holds for infinitely many security parameters $\secp\in \mathbb{N}$. 
\end{definition}

Next, we define
(infinitely-often) one-shot signatures. We focus on the case of single-bit messages for simplicity. The message space can be extended to multiple bits by a simple parallel repetition as shown in \cite{STOC:AGKZ20}.

\minki{We may need to write the classical and quantum state consistently; two notions $\sk$ and $\vk$ are a bit confusing.}\takashi{I changed the font for $\sk$. IS this good?}
\begin{definition}[One-shot signatures]\label{def:OSS}
A one-shot signature scheme consists of algorithms $(\setup,\keygen,\sign,\vrfy)$.
\begin{description}
\item[$\setup(1^\secp)\rightarrow \crs$:] This is a PPT algorithm that takes the security parameter $1^\secp$ as input, and outputs a classical public parameter $\pp$.
\item[$\keygen(\pp)\rightarrow (\vk,\qsk)$:] This is a QPT algorithm that takes a public parameter $\pp$ as input, and outputs a classical verification key $\vk$ and a quantum signing key $\qsk$.
\item[$\sign(\pp,\qsk,b)\rightarrow \sigma$:] This is a QPT algorithm that takes a public parameter $\pp$, a signing key $\qsk$ and a message $b\in \bit$ as input, and outputs a classical signature $\sigma$. 
\item[$\vrfy(\pp,\vk,b,\sigma)\rightarrow \top/\bot$:] This is a PPT algorithm that takes a public parameter $\pp$, a verification key $\vk$, a message $b$, and a signature $\sigma$ as input, and outputs the decision $\top$ or $\bot$.
\end{description}
We require a one-shot signature scheme to satisfy the following properties.

\smallskip
\noindent\textbf{Correctness.}
For any $b\in \bit$, we have 
\begin{align*}
    \Pr\left[\vrfy(\pp,\vk,b,\sigma)\rightarrow \top 
    :
    \pp\gets \setup(1^\secp),
    (\pk,\qsk)\gets\keygen(\pp),
    \sigma\gets \sign(\pp,\qsk,b)
    \right]= 1-\negl(\secp).
\end{align*}

\smallskip
\noindent\textbf{(Infinitely-often) Security.}
We say that a one-shot signature scheme is secure 
if for any non-uniform QPT adversary $\A$, we have 
\begin{align*}
    \Pr\left[
    \forall b\in \bit~\vrfy(\pp,\vk,b,\sigma_b)=\top
    :
    \pp\gets \setup(1^\secp),
    (\vk,\sigma_0,\sigma_1)\gets \A(\pp)
    \right]=\negl(\secp).
\end{align*}

We say that it is infinitely-often secure if the above holds for infinitely many security parameters $\secp\in \mathbb{N}$. 
\end{definition}

Then, we give a proof of \Cref{lem:Gap_OW_and_EOW}.

\begin{proof}[Proof of \Cref{lem:Gap_OW_and_EOW}]
Sinc the proof is almost identical for both \Cref{item:gap_one,item:gap_two}, we first prove \Cref{item:gap_one} and then explain how to modify it to prove \Cref{item:gap_two}. 

\smallskip
\noindent\textbf{Proof of \Cref{item:gap_one}.}
Let $(G,S,\star)$ be a group action with efficient algorithms that is one-way but not infinitely-often uniform extended one-way. Then, there is a uniform QPT algorithm $\A$ and a polynomial $\poly$ such that 
\begin{align}
\label{eq:break_eow}
    \Pr\left[
    h'\star t = h\star s
    :
    \begin{array}{l}
     s\gets S,
    g,h\gets G,
    t  := g \star s,
    h' \leftarrow \A(s,t,\ket{hG_{s}})
    \end{array}
    \right] > 1/\poly(\secp)
\end{align}
for all $\secp$. 
Then, we construct a one-shot signature scheme as follows. Let $N\seteq \poly(\secp)\cdot \secp$. 

\begin{description}
\item[$\setup(1^\secp)$:] For $i\in [N]$, generate $s_i\gets S$, $g_i\gets G$, set $t_i \seteq g_i\star s_i$, and output
$\pp\seteq \{s_i,t_i\}_{i\in [N]}$.
\item[$\keygen(\pp)$:] 
Given $\pp=\{s_i,t_i\}_{i\in [N]}$, 
for $i\in [N]$, 
generate 
\begin{align*}
    \ket{G}=\frac{1}{|G|^{1/2}}\sum_{h\in G}\ket{h}, 
\end{align*}
coherently compute the group action on $s_{i}$ in another register to get 
\begin{align*}
    \frac{1}{|G|^{1/2}}\sum_{h\in G}\ket{h}\ket{h\star s_i}, 
\end{align*}
measure the second register to get $u_i$. At this point, the first register collapses to $h_i G_{s_i}$ \mor{$|h_iG_{s_i}\rangle$?} for $h_i$ such that $h_i\star s_i =u_i$.\footnote{Remark that $h_i G_{s_i}$ only depends on $u_i$.}   
Output $\vk\seteq \{u_i\}_{i\in \secp}$ \mor{$i\in[N]$?} and $\qsk\seteq \{u_i,\ket{h_i G_{s_i}}\}_{i\in[N]}$. 

\item[$\sign(\pp,\qsk,b)\rightarrow \sigma$:] 
Given $\pp=\{s_i,t_i\}_{i\in [N]}$, $\qsk= \{u_i,\ket{h_i G_{s_i}}\}_{i\in[N]}$, and $b\in \bit$, do the following.
\begin{itemize}
    \item If $b=0$, for $i\in [N]$, measure $\ket{h_i G_{s_i}}$ to get $\tilde{h}_i\in h_i G_{s_i}$ and output $\sigma\seteq \{\tilde{h}_i\}_{i\in [N]}$.
    \item If $b=1$, for $i\in [N]$, run $\A(s_i,t_i,\ket{h_i G_{s_i}})$ to get $h'_i$. If $h'_i \star t_i \neq u_i$ for all $i\in [N]$, it aborts. Otherwise, it outputs $\sigma \seteq (i^*,h'_{i^*})$ where $i^*$ is the smallest index such that $h'_{i^*}\star t_{i^*}=u_{i^*}$. 
\end{itemize}
\item[$\vrfy(\pp,\vk,b,\sigma)\rightarrow \top/\bot$:] Given $\pp=\{s_i,t_i\}_{i\in [N]}$, $\vk=\{u_i\}_{i\in \secp}$\mor{$i\in[N]$?}, $b\in \bit$, and a signature $\sigma$, do the following.
\begin{itemize}
    \item If $b=0$, parse $\sigma=\{\tilde{h}_i\}_{i\in [N]}$, and output $\top$ if $\tilde{h}_i\star s_i = u_i$ for all $i\in [N]$ and $\bot$ otherwise. 
    \item If $b=1$, parse $\sigma=(i,h'_i)$, and output $\top$ if $h'_i \star t_i = u_i$ and $\bot$ otherwise. 
\end{itemize}
\end{description}

\noindent\textbf{Correctness.}
It is easy to see that the signing algorithm outputs a valid signature whenever it does not abort. By \Cref{eq:break_eow}, the probability that the signing algorithm abort (when $b=1$) is 
\begin{align*}
    (1-1/\poly)^{N} = \negl(\secp)
\end{align*}
by $N= \poly(\secp)\cdot \secp$.
\takashi{Wait, this holds only for inifinitely many $\secp$. I need to think about it later. Probably, we should have started from the assumption that the group action is not inifinitely-often uniform extended one-way.}
\minki{I briefly checked the proof and it seems to be correct. Are you concern if the notion of infinitely-often is usually considered for the security in the literature? I think it is okay to just define the infinite-often correctness.}
\minki{I briefly checked~\cite{EC:Zhandry19b}, and it seems that the quantum lightning scheme is also infinitely-often correct if the hash function is just not-collapsing.}
\takashi{
That point is ambiguous in his paper, but I believe we can also achieve infinitely-often \emph{security} from not-collapsing. The reason is that we can modify the verification algorithm so that it accepts everything on security parameters on which the adversary does not work. One non-triviality is if the verification algorithm can know a given security parameter is good for the adversary. But this is fine since the verifier can estimate the adversary's success probability up to a 1/poly error by running it polynomially many times. But this is somewhat complicated to explain, so I think it would be easier to focus on the other flavor of the theorem, i.e., assuming not infinitely-often extended one-way, and construct normal one-shot signatures. 
}
\takashi{I resolved the issue.}

\smallskip
\noindent\textbf{Security.}
Suppose that there is a non-uniform QPT adversary that breaks the above one-shot signature scheme. The adversary is given $\pp=\{s_i,t_i\}_{i\in [N]}$ and  
finds 
$\vk=\{u_i\}_{i\in [N]}$,
$\sigma_0=\{\tilde{h}_i\}_{i\in [N]}$,  and
$\sigma_1=(i^*,h'_{i^*})$ such that 
$\tilde{h}_i\star s_i = u_i$ for all $i\in [N]$ and 
$h'_{i^*} \star t_{i^*} = u_{i^*}$ 
with a non-negligible probability. 
In particular, 
when the above happens, we have $\tilde{h}_{i^*}\star s_{i^*}=h'_{i^*} \star t_{i^*}$. 
Thus, if we set $g'_{i^*}\seteq {h'_{i^*}}^{-1}\tilde{h}_{i^*}$, then we have $g'_{i^*}\star s_{i^*} = t_{i^*}$. 
Thus, by randomly guessing $i^*$ and embedding a problem instance of the one-wayness into the $i^*$-th coordinate, we can break the one-wayness of $(G,S,\star)$, which is a contradiction. 
Thus, the above one-shot signature scheme is secure.

This completes the proof of \Cref{item:gap_one}.

\smallskip
\noindent\textbf{Proof of \Cref{item:gap_two}.}
The proof is similar to that of \Cref{item:gap_one}. The difference is that since we only assume $(G,S,\star)$ is not uniform extended one-way, we can only assume that \Cref{eq:break_eow} holds for infinitely many $\secp$ rather than all $\secp$. In this case, the correctness of the above one-shot signature scheme only holds for infinitely many $\secp$. To deal with this, we modify the verification algorithm %to estimate $\A$'s success probability and just accept regardless of $\sigma$ when the approximated success probability is small. More precisely, let $p(\secp)$ be the probability that 
so that it approximates $\A$'s success probability up to additive error $1/(4\poly(\secp))$ (except for a negligible probability) and simply accepts if the approximated success probability is smaller than $1/(2\poly(\secp))$. 
Then, the correctness holds on all $\secp\in \mathbb{N}$ because
\begin{itemize}
    \item if the real success probability is smaller than $1/(4\poly(\secp))$, the estimated success probability is smaller than $1/(2\poly(\secp))$ with overwhelming probability, and thus the verification algorithm accepts with overwhelming probability on these security parameters, and
    \item if the real success probability is smaller than $1/(4\poly(\secp))$, the signing algorithm should succeed in generating a valid proof with overwhelming probability and thus the  verification algorithm accepts with overwhelming probability on these security parameters. 
\end{itemize}
For the security, we observe that the estimated success probability is smaller than $1/(2\poly(\secp))$ with a negligible probability when the real success probability is larger than $1/\poly(\secp)$. Thus, for those security parameters, the adversary should find valid signatures in the original scheme. Since there are infinitely many such $\secp$, this is not possible by the one-wayness of $(G,S,\star)$. 
%to always accept on security parameters on which \Cref{eq:break_eow} does not hold.\takashi{I found a problem here. The verification algorithm cannot know if  \Cref{eq:break_eow} holds. I said estimation should work, but then there's a inverse polynomial error, which looks problematic. An alternative approach is to simply hardwire into the verification algorithm the one-bit information if the security parameter satisfies  \Cref{eq:break_eow}, but this results in \emph{non-uniform} verification algorith. Then, I'm not sure how to prove \Cref{item:gap_two}. Probably, we can just delete this claim, or only consider infinitely-often \emph{correctness} as suggested by Minki.}
\end{proof}

\subsection{Quantum-Ciphertext Public Key Encryption from Group Actions}\label{sec:QPKE_from_GA_app}
Here, we give a complete discription of the quantum-ciphertext PKE scheme based on group actions constructed in \Cref{sec:QPKE_from_GA}. 

Let $(G,S,\star)$ be a group action with efficient algorithms as defined in \Cref{def:GA_efficient}. 
%For simplicity, we describe the scheme as if a uniform superposition over $G$ can be generated (instead of negligibly close one as required in \Cref{def:GA_efficient}), but the same construction and proof works without assuming this noting that no quantum algorithm distinguishes two quantum states with advantage larger than their trace distacne. 
Our construction of quantum PKE scheme is described as follows.

\begin{description}
\item[$\keygen(1^\secp)$:] 
Choose $s_0\gets S$ and $g\gets G$, set $s_1\seteq g\star s_0$, and output $\pk\seteq (s_0,s_1)$ and $\sk \seteq g$. 
\item[$\enc(\pk,b\in \bit)$:] 
Parse $\pk=(s_0,s_1)$. 
Generate a state  
\begin{align*}
    \frac{1}{\sqrt{2}}(\ket{0}+(-1)^b\ket{1})\ket{G} =
    \frac{1}{\sqrt{2}}(\ket{0}+(-1)^b\ket{1})\sum_{h\in G}\ket{h},
\end{align*}
coherently compute the group action on $s_0$ or $s_1$ controlled by the first qubit in an additional register to get 
\begin{align*}
    \sum_{h\in G}\frac{1}{\sqrt{2}}(\ket{0}\ket{h}\ket{h \star s_0}+(-1)^b \ket{1}\ket{h}\ket{h\star s_1}),
\end{align*}
and measure the rightmost register to get $u\in S$. At this point, the first two registers collapse to \begin{align*}
    \frac{1}{\sqrt{2}}(\ket{0}\ket{h G_{s_0}}+(-1)^b \ket{1}\ket{h G_{s_0} g^{-1}}),
\end{align*}
for $h\in G$ such that $h \star s_0 =u$.\footnote{Note that there may be multiple such $h$ but $h G_{s_0}$ does not depend on the choice of $h$.}
The above state is set to be $\qct$. 
\item[$\dec(\sk,\qct)$:]
Parse $\sk=g$. 
Let $\regD$ and $\regG$ be the first and second registers of $\qct$, respectively. 
Prepare $\ket{+}_\regB=\frac{1}{\sqrt{2}}(\ket{0}+\ket{1})_\regB$ in an additional one-qubit register $\regB$. 
Let $U_g$ be a unitary over $\regD$ and $\regG$ such that 
\begin{align*}
    &U_g \ket{0}_{\regD} \ket{h}_{\regG} = \ket{1}_{\regD}\ket{hg^{-1}}_{\regG}, \\
    &U_g \ket{1}_{\regD}\ket{h}_{\regG} = \ket{0}_{\regD}\ket{hg}_{\regG}.
\end{align*}
Apply the controlled-$U_g$ controlled by $\regB$.
Finally, measure $\regB$ in the Hadamard basis and output the measurement outcome $b'$. (See Figure ?? \takashi{to be written.})
%it appends $\frac{1}{\sqrt{2}}(\ket{0}+\ket{1})$ on the top of $\ct$,   
%it runs the quantum circuit as described in Figure?? \takashi{to be written} to get a measurement outcome $b'$ and outputs $b'$.
\end{description}

The above scheme is IND-CPA secure assuming that $(G,S,\star)$ is extended one-way by \Cref{cor:QPKE_and_equ,thm:equ_from_eow}.

\if0
\noindent\textbf{Correctness}
First, we show the correctness. 
\begin{theorem}
$\QPKE$ satisfies the correctness.
\end{theorem}
\begin{proof}
It is easy to see that $U_g$ satisfies the following:
\begin{align*}
    &U_g \ket{0}_{\regD} \ket{hG_s}_{\regG} = \ket{1}_{\regD}\ket{hG_s g^{-1}}_{\regG}, \\
    &U_g \ket{1}_{\regD}\ket{hG_s g^{-1}}_{\regG} = \ket{0}_{\regD}\ket{hG_s}_{\regG}.
\end{align*}
This immediately implies the following:
\begin{align*}
    &U_g \frac{1}{\sqrt{2}}(\ket{0}_{\regD}\ket{h G_s}_{\regG}+\ket{1}_{\regD}\ket{h G_s g^{-1}}_{\regG})=\frac{1}{\sqrt{2}}(\ket{0}_{\regD}\ket{h G_s}_{\regG}+\ket{1}_{\regD}\ket{h G_s g^{-1}}_{\regG}), \\
    &U_g \frac{1}{\sqrt{2}}(\ket{0}_{\regD}\ket{h G_s}_{\regG}-\ket{1}_{\regD}\ket{h G_s g^{-1}}_{\regG})=-\frac{1}{\sqrt{2}}(\ket{0}_{\regD}\ket{h G_s}_{\regG}-\ket{1}_{\regD}\ket{h G_s g^{-1}}_{\regG}).
\end{align*}
Thus, when the decryption algorithm runs on $\sk=g$ and $\ct= \frac{1}{\sqrt{2}}(\ket{0}\ket{h G_s}+(-1)^b \ket{1}\ket{h G_s g^{-1}})$, the state before the measurement is
\begin{align*}
    \frac{1}{\sqrt{2}}
\end{align*}
\end{proof}

\noindent\textbf{Security}
The following theorem asserts the security of 
\fi
